# Supplementary material for: The $SL(2,\mathbb{Z})$ dualization algorithm at work
Source: arXiv:2212.10571 source file (2023-03-14)
Supplement: Supplementary file 1 [file 11_Sdual_proof.pdf]

$$\sqrt{pqt}^{\frac{N-M+1}{2}-j} cd \quad \text{[Diagram: A box labeled 2 with a blue shaded region above it and a green line connecting it to the left side of the equation]} \quad u \quad \times \prod_{j=1}^{N-M} \frac{\Gamma_e(t^{1-j} c^2)}{\Gamma_e(t^{1-j} d^{-2})}$$

$$\times \prod_{j=1}^{N-M} \frac{\Gamma_e(t^{1-j}c^2)}{\Gamma_e(pqt^{-j})}$$

$$\times \prod_{j=1}^{N-M} \frac{\Gamma_e(t^{1-j}c^2)}{\Gamma_e(pqt^{-j})}$$

$$t^{\frac{M-N+1}{2}} d^{-1} \sqrt{pq} t^{\frac{N-M}{2}}$$

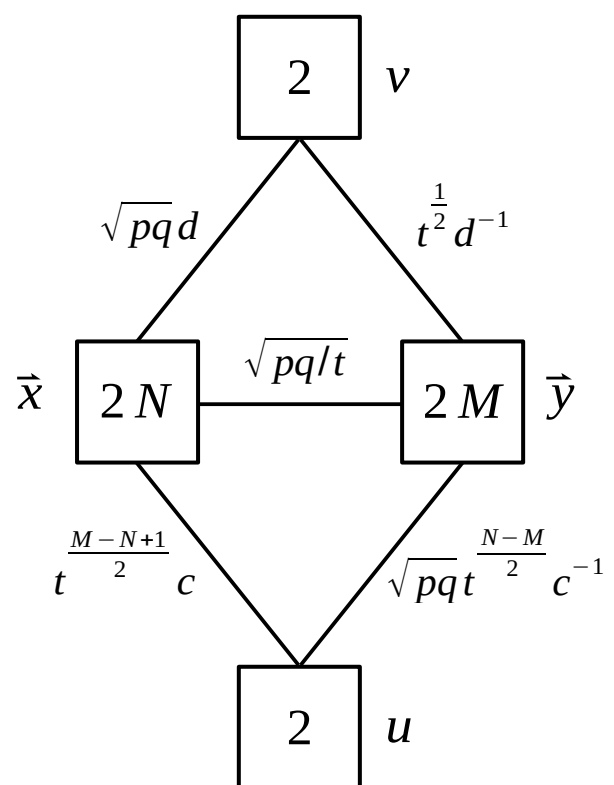

=

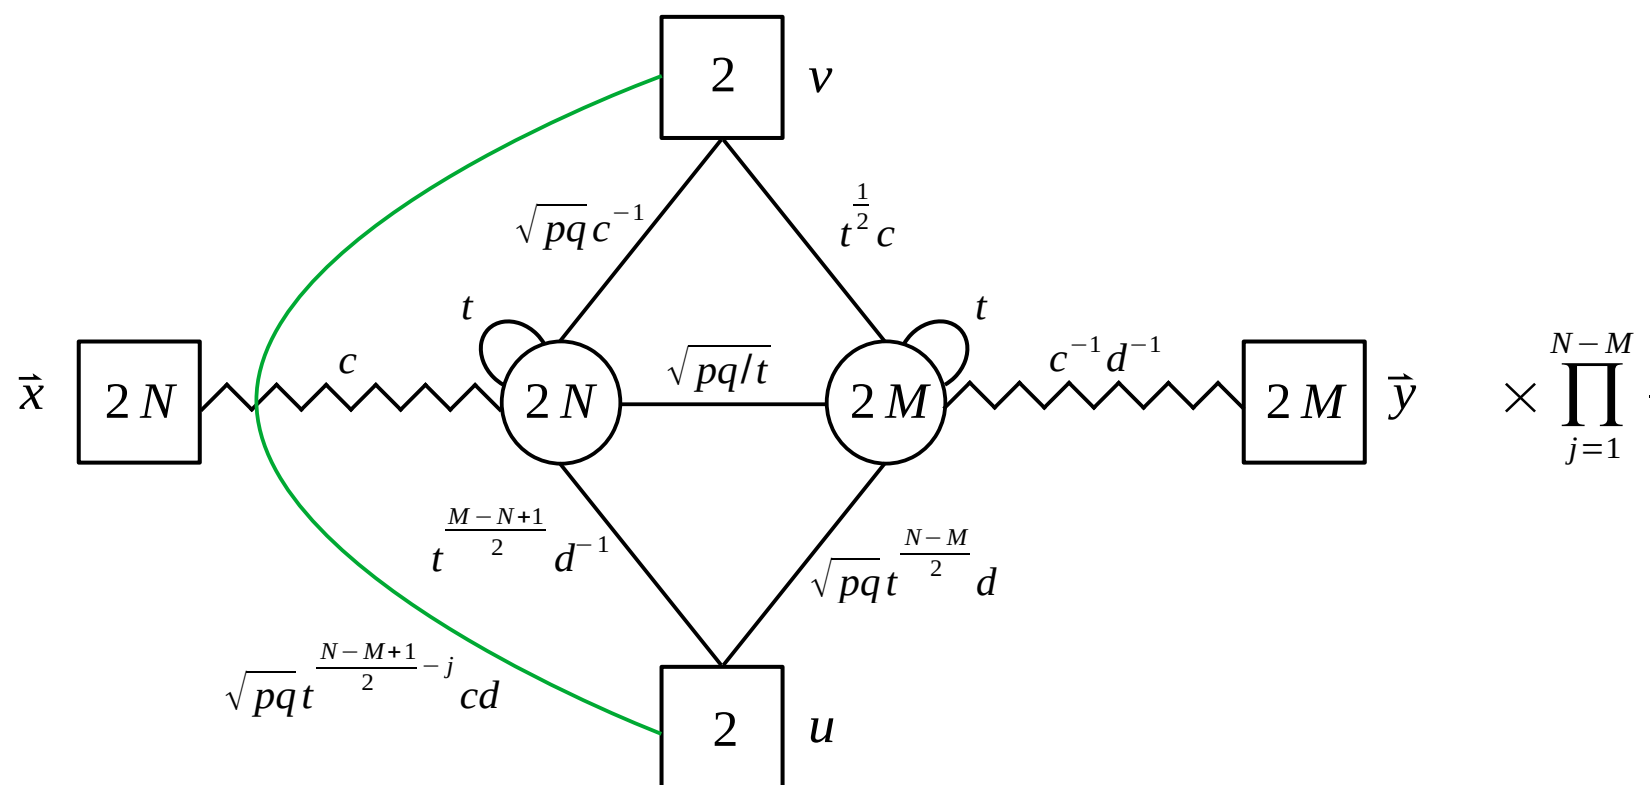

$\times \prod_{j=1}^{N-M}$
